# Supplementary material for: Inversion symmetry breaking induced triply degenerate points in orderly arranged PtSeTe family materials
Source: arXiv:1803.01134 ancillary file (2018-03-03)
Supplement: Supplementary file 1 [file SupM.pdf]

# Supplemental Material for "Inversion symmetry breaking induced triply degenerate points in orderly arranged PtSeTe family materials"

R. C. Xiao,[1,2,*] C. H. Cheung,[3,*] P. L. Gong,[4] W. J. Lu,[1,†] J. G. Si,[1,2] and Y. P. Sun[1,5,6,‡]

[1]*Key Laboratory of Materials Physics, Institute of Solid State Physics, Chinese Academy of Sciences, Hefei 230031, China*
[2]*University of Science and Technology of China, Hefei 230026, China*
[3]*Graduate Institute of Applied Physics, National Taiwan University, Taipei 10617, Taiwan*
[4]*Department of Physics, Southern University of Science and Technology, Shenzhen 518055, China*
[5]*High Magnetic Field Laboratory, Chinese Academy of Sciences, Hefei 230031, China*
[6]*Collaborative Innovation Center of Microstructures, Nanjing University, Nanjing 210093, China*

## I. CHARACTER TABLE OF $C_{3v}$

Character table for point group $C_{3v}$ is shown in Table S1, and Mulliken symbols ($A_1$, $A_2$, $E$) for some irreducible representations are also listed.

TABLE S1: Character table for double point group $C_{3v}$.

| $C_{3v}/3m$ | $\mathbb{I}$ | $\overline{\mathbb{I}}$ | $2C_3$ | $2\overline{C_3}$ | $3\sigma_v$ | $3\overline{\sigma_v}$ | Bases |
|---|---|---|---|---|---|---|---|
| $\Gamma_1/A_1$ | 1 | 1 | 1 | 1 | 1 | 1 | $z$ |
| $\Gamma_2/A_2$ | 1 | 1 | 1 | 1 | -1 | -1 | $S_z$ |
| $\Gamma_3/E$ | 2 | 2 | -1 | -1 | 0 | 0 | $(x, y)$ |
| $\Gamma_4$ | 2 | -2 | 1 | -1 | 0 | 0 | $\{\vert 1/2, 1/2\rangle, \vert 1/2, -1/2\rangle\}$ |
| $\Gamma_5$ | 1 | -1 | -1 | 1 | i | -i | $(\vert 3/2, -3/2\rangle - i\vert 3/2, 3/2\rangle)$ |
| $\Gamma_6$ | 1 | -1 | -1 | 1 | -i | i | $(i\vert 3/2, -3/2\rangle - \vert 3/2, 3/2\rangle)$ |

Note: data are from Ref. 1. $\mathbb{I}$ means identity, $S_z$ stands for the $z$ competent of an axial vector ($\mathbf{S} = \mathbf{r} \times \mathbf{p}$).

According to the above table:

$$\begin{cases} A_1 \otimes D^{1/2} = \Gamma_4, \\ A_2 \otimes D^{1/2} = \Gamma_4, \\ E \otimes D^{1/2} = \Gamma_4 \oplus \Gamma_5 \oplus \Gamma_6, \end{cases} \tag{S1}$$

where $D^{1/2}$ is the representation matrix of spin. From Eq. S1, we can see that $A_1/A_2$ state transfers into $\Gamma_4$, while $E$ state splits into $\Gamma_4$, $\Gamma_5$, and $\Gamma_6$ sates when spin orbit coupling (SOC) effects are considered. $\Gamma_5$ and $\Gamma_6$ transfer into each other under the time reversal operator $T$:

$$\begin{cases} T\Gamma_5 = -\Gamma_6, \\ T\Gamma_6 = \Gamma_5, \end{cases} \tag{S2}$$

and the matrix of time reversal operator for the bases of $(\Gamma_5, \Gamma_6)$ is

$$D(T) = \begin{pmatrix} 0 & 1 \\ -1 & 0 \end{pmatrix} K, \tag{S3}$$

where $K$ is complex conjugate operator. Therefore, these two states are Kramers pair, and they are degenerate at time reversal symmetry point. Along the $\Gamma - A$ ($\Delta$) path, we prefer $\Delta_4$, $\Delta_5$, and $\Delta_6$ instead of $\Gamma_4$, $\Gamma_5$, and $\Gamma_6$.

## II. $k \cdot p$ DERIVATION

The little group of $A$ point is $C_{3v} \otimes 1'$ ($1' = \{\mathbb{I}, T\}$). There are two generators of $C_{3v}$ including a threefold rotational symmetry $C_{3z}(-x/2-\sqrt{3}y/2, \sqrt{3}x/2-y/2, z)$ and mirror symmetry $\sigma_{yz}(-x, y, z)$. Consequently, the related symmetry representation matrices under the bases of $\{\Delta_4, \Delta_5, \Delta_6\}$ are given by

$$D(C_{3z}) = \begin{pmatrix} e^{i\pi/3} & 0 \\ 0 & e^{-i\pi/3} \end{pmatrix} \oplus \begin{pmatrix} -1 & 0 \\ 0 & -1 \end{pmatrix}, \tag{S4}$$

$$D(\sigma_{yz}) = \begin{pmatrix} 0 & i \\ i & 0 \end{pmatrix} \oplus \begin{pmatrix} i & 0 \\ 0 & -i \end{pmatrix}, \tag{S5}$$

$$D(T) = \begin{pmatrix} 0 & 1 \\ -1 & 0 \end{pmatrix} K \oplus \begin{pmatrix} 0 & 1 \\ -1 & 0 \end{pmatrix} K. \tag{S6}$$

According to invariant theory:

$$D(R)H(\mathbf{k})D(R)^{-1} = H(R\mathbf{k}), \tag{S7}$$

where $R$ is a symmetry operator, the derived effective Hamiltonian around $A$ point that considers first-order $k$ terms for off-diagonal matrix elements and second-order $k$ terms for diagonal matrix elements is:

$$H_{eff}(\mathbf{q}) = \varepsilon_0(\mathbf{q}) + \begin{bmatrix} M(\mathbf{q}) & iCq_+ & Aq_- & -A^*q_- \\ -iCq_- & M(\mathbf{q}) & -Aq_+ & -A^*q_+ \\ A^*q_+ & -A^*q_- & -M(\mathbf{q}) + Bq_z & 0 \\ -Aq_+ & -Aq_- & 0 & -M(\mathbf{q}) - Bq_z \end{bmatrix}, \tag{S8}$$

where $\varepsilon_0(\mathbf{q}) = C_0 + C_1q_z^2 + C_2(q_x^2 + q_y^2)$, $M(\mathbf{q}) = M_0 - M_1q_z^2 - M_2(q_x^2 + q_y^2)$, $\mathbf{q} = \mathbf{k} - \mathbf{A}$, $q_+ = q_x + iq_y$, and $q_- = q_x - iq_y$. $A$ is a complex number, while $B$ and $C$ are real numbers.

## III. CHIRALITY OF EACH TDP

By using similar method that drives $k \cdot p$ effective Hamiltonian near $A$ point, we can get the effective Hamiltonian near the TDPs. The 3×3 effective Hamiltonian around the TDP ($T1$) by $\Delta_4$ and $\Delta_5$ bands keeping only linear order terms for matrix elements is as follows:

$$H_{\Delta_4,\Delta_5} = \eta p_z + \begin{bmatrix} \alpha p_z & i\beta p_+ & \gamma p_- \\ -i\beta p_- & \alpha p_z & -\gamma p_+ \\ \gamma^* p_+ & -\gamma^* p_- & -\alpha p_z \end{bmatrix}, \tag{S9}$$

where $\mathbf{p} = \mathbf{q} - \mathbf{q}_{T1} = (p_x, p_y, p_z)$, $\alpha$, $\beta$ and $\eta$ are real numbers, and $\gamma$ is a complex number.

The 2×2 Hamiltonian of the crossing point of $\Delta_{4\uparrow}$ and $\Delta_5$ is:

$$H_{\Delta_4\uparrow,\Delta_5} = \eta p_z + \begin{bmatrix} \alpha p_z & \gamma p_- \\ \gamma^* p_+ & -\alpha p_z \end{bmatrix}, \tag{S10}$$

and the effective Hamiltonian of the crossing point of $\Delta_{4\downarrow}$ and $\Delta_5$ is:

$$H_{\Delta_4\downarrow,\Delta_5} = \eta p_z + \begin{bmatrix} \alpha p_z & -\gamma p_+ \\ -\gamma^* p_- & -\alpha p_z \end{bmatrix}. \tag{S11}$$

Any 2×2 Hermitian matrix can be expanded by the Pauli matrices and the identity matrix:

$$H = \sum_i \sigma_0 v_{0i} p_i + \sum_{i,j} v_{ij} p_i \sigma_j, \tag{S12}$$

where $\sigma_0$ is a 2×2 identity matrix, $i, j = x, y, z$, $\sigma_j$ are one of three Pauli matrices. So Eq. S10 can be rewrote as:

$$H_{\Delta_{4\uparrow},\Delta_5} = \eta p_z\sigma_0 + p_z\alpha\sigma_z + p_x\gamma_R\sigma_x + p_y\gamma_R\sigma_y - p_x\gamma_I\sigma_y + p_y\gamma_I\sigma_x, \tag{S13}$$

and Eq. S11 can be rewrote as:

$$H_{\Delta_{4\downarrow},\Delta_5} = \eta p_z\sigma_0 + p_z\alpha\sigma_z - p_x\gamma_R\sigma_x + p_y\gamma_R\sigma_y + p_x\gamma_I\sigma_y + p_y\gamma_I\sigma_x, \tag{S14}$$

where $\gamma_R$ and $\gamma_I$ are the real and imaginary part of $\gamma$, respectively. So

$$V_{\Delta_{4\uparrow},\Delta_5} \equiv [v_{ij}]_{\Delta_{4\uparrow},\Delta_5} = \begin{bmatrix} \gamma_R & -\gamma_I & 0 \\ \gamma_I & \gamma_R & 0 \\ 0 & 0 & \alpha \end{bmatrix}, \tag{S15}$$

$$V_{\Delta_{4\downarrow},\Delta_5} \equiv [v_{ij}]_{\Delta_{4\downarrow},\Delta_5} = \begin{bmatrix} -\gamma_R & \gamma_I & 0 \\ \gamma_I & \gamma_R & 0 \\ 0 & 0 & \alpha \end{bmatrix}. \tag{S16}$$

According to Ref. 2, the chirality of a 2×2 Hamiltonian $\chi = sgn\left[det(V)\right]$, so

$$\chi(\Delta_{4\uparrow}, \Delta_5) = -\chi(\Delta_{4\downarrow}, \Delta_5). \tag{S17}$$

Similarly, the 3×3 effective Hamiltonian around the TDP by $\Delta_4$ and $\Delta_6$ bands is:

$$H_{\Delta_4,\Delta_6} = \eta' p_z + \begin{bmatrix} \alpha' p_z & i\beta' p_+ & \gamma' p_- \\ -i\beta' p_- & \alpha' p_z & \gamma' p_+ \\ \gamma'^* p_+ & \gamma'^* p_- & -\alpha' p_z \end{bmatrix}, \tag{S18}$$

where $\alpha'$, $\beta'$, and $\eta'$ are real numbers and $\gamma'$ is a complex number. Using similar method, we can prove that one TDP formed by $\Delta_4$ and $\Delta_6$ bands can also be viewed as two Weyl points with opposite chirality. Moreover, the results are invariant with the values of above $k \cdot p$ parameter. These results are similar with the TDPs induced by breaking time reversal symmetry in centrosymmetric system.[3]


* The authors contributed equally to this work.
† Electronic address: wjlu@issp.ac.cn
‡ Electronic address: ypsun@issp.ac.cn


1 G. F. Koster, *Properties of the thirty-two point groups*, The MIT Press (1963).
2 X. Wan, A. M. Turner, A. Vishwanath, and S. Y. Savrasov, Phys. Rev. B **83**, 205101 (2011).
3 C. H. Cheung, R. C. Xiao, M. C. Hsu, H. R. Fuh, Y. C. Lin, and C. R. Chang, arXiv:1709.07763.
